# Supplementary material for: Solving Large Steiner Tree Problems in Graphs for Cost-Efficient Fiber-To-The-Home Network Expansion
Source: arXiv:2109.10617 source file (2021-11-24)
Supplement: Supplementary file 1 [file appendix.tex]

\section*{\uppercase{Appendix}}

\begin{center}
\begin{table}[htbp]
{\small
\begin{center}
\begin{tabular}{l p{3.5cm}}
\toprule
\textbf{Method} & \textbf{Description} \\
\midrule
\textbf{Simplifier} &\\
Triangle Simplifier & Uses an EA to simplify the graph. The objective function has two terms, a quality term and a size term. Weights for both terms can be selected.\\ 
Growing Neural Gas & Growing Neural Gas approach for graph simplification.\\ 
Physarum & Works similar to Physarum Solver.\\

\textbf{Partitioner} & \\
Greedy Modularity & Finds graph partitions that maximize modularity.\\ 
Spectral Clustering & Uses Spectral Clustering for graph partitioning.\\
Voronoi Partitioning & Partitions the input graph in Voronoi cells.\\

\textbf{Solver} & \\
Baseline (NetworkX) & Approximate Steiner Tree algorithm as implemented in the NetworkX Library.\\ 
Evolutionary Algorithm & Uses an Evolutionary Algorithm to find the best combinations of terminals (always all are used), non-terminals and their connections.\\
Physarum & Uses a nature-inspired heuristic based on the Physarum Polycephalum slime mold.\\
Quantum Annealing & Uses a QUBO formulation of the Steiner Tree problem suitable for Quantum Annealing.\\ 
Simulated Annealing & Uses a solver based on a Simulated Annealing and Metropolis approach.\\
\bottomrule
\end{tabular}
\end{center}
} % end of tiny
\caption[Overview: Simplifier, Partitioner, Solver]{Overview}\label{tab:overview}
\end{table}
\end{center}
